# Supplementary material for: PT-Symmetric Magnon Lasing and Anti-Lasing
Source: arXiv:2511.12165 source file (2025-11-15)
Supplement: Supplementary file 1 [file Supplementary_Material.pdf]

# Supplementary Material: $\mathcal{PT}$-Symmetric Magnon Lasing and Anti-Lasing

Xi-guang Wang[1], Tian-xiang Lu[2], Guang-hua Guo[1], Jamal Berakdar[3*], Hui Jing[4*]

[1] *School of Physics, Central South University, Changsha 410083, China*

[2] *College of Physics and Electronic Information, Gannan Normal University, Ganzhou 341000, China*

[3] *Institut für Physik, Martin-Luther Universität Halle-Wittenberg, 06099 Halle/Saale, Germany*

[4] *Key Laboratory of Low-Dimensional Quantum Structures and Quantum Control of Ministry of Education, Department of Physics and Synergetic Innovation Center for Quantum Effects and Applications, Hunan Normal University, Changsha 410081, China*

[*] *email: jamal.berakdar@physik.uni-halle.de; jinghui@hunnu.edu.cn*

(Dated: November 15, 2025)

## I. TUNING THE BRAGG POINT BY PERIOD LENGTH

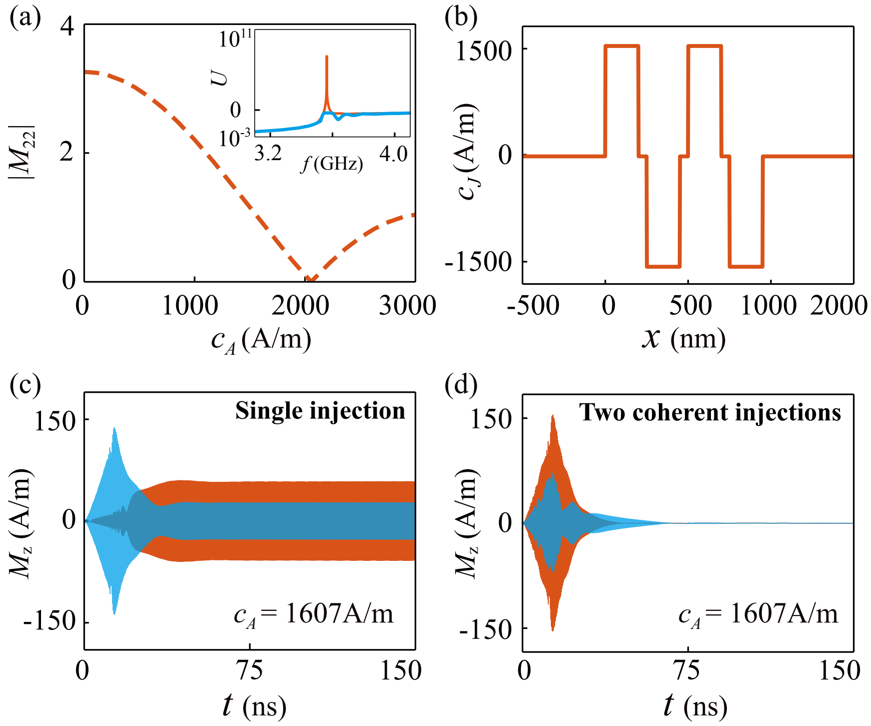


FIG. S1. (a) With $\Lambda = 500$ nm and $L = 1000$ nm, $M_{22}$ dependence on $c_{\rm A}$. The inset is the frequency dependent $U$ (logarithmic scale) under single injection and two coherent injections. Adopting the step function in (b), the numerically simulated time dependent $M_{\rm z}(t)$ profiles at $x = -200$ nm (blue curve) and $x = 1200$ nm (red curve) under (c) single injection and (d) two coherent injections. Two coherent microwave field pulses $h_0 \sin(2\pi f t)\mathbf{z}$ (c) and $h_1 \sin(2\pi f t + \phi)\mathbf{z}$ (added to d) are applied at $x = -1000$ nm and $x = 2000$ nm, respectively. Here, pulse duration is 10 ns, $h_1/h_0 = 0.46$, $h_0 = 1000$ A/m, $\phi = -1.3$ and $f = 3.56$ GHz.

The magnon laser frequency can be tuned by changing the Bragg point. As an example, for periodic sine function $c_{\rm J}(x) = c_{\rm A} \sin(2k_{\rm p}x)$ with period length $\Lambda = 500$ nm and $L = 1000$ nm in Fig. S1(a), the Bragg point frequency becomes 3.56 GHz, and at this frequency the magnon laser condition is fulfilled for the electric current amplitude $c_{\rm A} = 2055$ A/m under the sin function potential. Using a step function $c_{\rm J}(x)$ of Fig. S1(b) to realize the laser structure, only four separated charge-carrying stripes are enough, which is a much simpler structure than that suggested in main article. The lasing effect is proved by numerical simulations in Fig. S1(c), where the critical value $c_{\rm A} = 1607$ A/m can drive the unattenuated

magnons under pulsed excitation. With constant injection the laser amplification leads to very large amplitude after a long duration (not shown). Also, with two coherent injections, the magnon pulse is totally suppressed in Fig. S1(d). These results validate the effectiveness of the simpler structure for the magnon laser absorber.

## II. MAGNONIC LASING AND ANTI-LASING IN ANTIFERROMAGNET

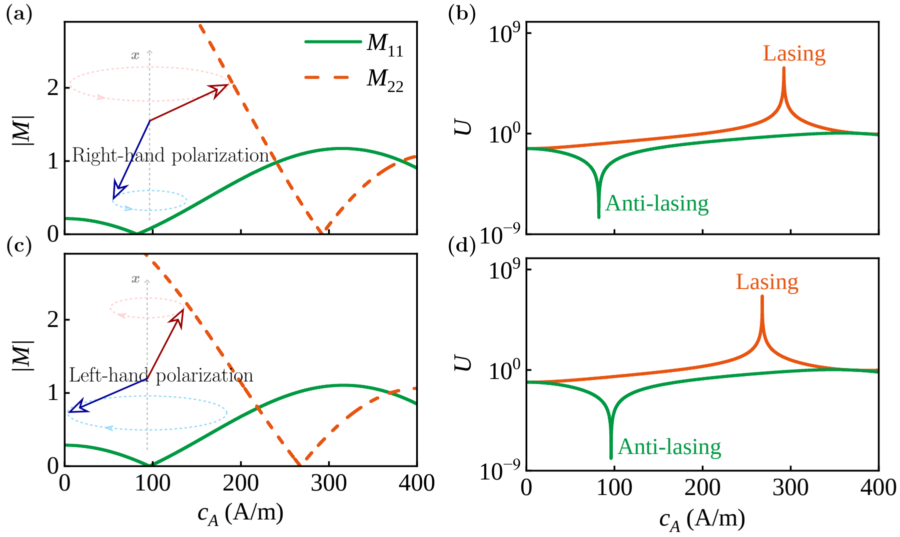


FIG. S2. For the AFM layer and periodic SOT with $\Lambda = 50$ nm and $L = 2000$ nm, $M_{11}$, $M_{22}$ and $U$ (logarithmic scale) dependence on the electric current amplitude $c_{\rm A}$ of right-hand (a-b, frequency $\Re[\omega_+/2\pi] = 0.296$ THz) and left-hand (c-d, frequency $\Re[\omega_-/2\pi] = -0.24$ THz) polarized magnons. Material parameters for $MnF_2$ are used in the calculations for Eq. (S4): $\omega_{\rm E} = 9.3$ THz, $\omega_{\rm A} = 0.15$ THz, $\omega_{\rm H} = 0.176$ THz, $\alpha = 0.00002$ and $a = 4.1$Å. Red and blue arrows represent the sublattice magnetizations $\mathbf{m}_1$ and $\mathbf{m}_2$ respectively.

The lasing and anti-lasing mechanism also applies to antiferromagnet (AFM) magnons within THz frequency range. AFM hosts two degenerate magnon modes with opposite angular momenta. The application of AFM magnons entails a symmetry break between two opposite modes[1–4]. Here, by applying an external magnetic field, the degeneracy of lasing and anti-lasing conditions of two modes are lifted, allowing for the selective excitation of one polarized mode. To construct the analytic model for AFM, wo introduce the average magnetization vector $\mathbf{m} = (\mathbf{m}_1 + \mathbf{m}_2)/2$ and the Néel vector $\mathbf{n} = (\mathbf{m}_1 - \mathbf{m}_2)/2$. Here, $\mathbf{m}_1$

and $\mathbf{m}_2$ represent sublattice magnetization of the AFM. The coupled LLG equations for $\mathbf{m}$ and $\mathbf{n}$ are [1, 2],

$$\begin{aligned}\partial_{\rm t}\mathbf{m} &= (\boldsymbol{\omega}_{\rm m}\times\mathbf{m}+\boldsymbol{\omega}_{\rm n}\times\mathbf{n})/2+\alpha(\mathbf{m}\times\partial_{\rm t}\mathbf{m}+\mathbf{n}\times\partial_{\rm t}\mathbf{n})+\mathbf{T}_{\rm m},\\ \partial_{\rm t}\mathbf{n} &= (\boldsymbol{\omega}_{\rm m}\times\mathbf{n}+\boldsymbol{\omega}_{\rm n}\times\mathbf{m})/2+\alpha(\mathbf{m}\times\partial_{\rm t}\mathbf{n}+\mathbf{n}\times\partial_{\rm t}\mathbf{m})+\mathbf{T}_{\rm n}.\end{aligned}\tag{S1}$$

The effective field frequencies $\boldsymbol{\omega}_{\rm m(n)}$ are defined by $\boldsymbol{\omega}_{\rm m(n)}=-\frac{\gamma}{M_{\rm s}}\frac{\delta E_{\rm AFM}}{\delta\mathbf{m(n)}}$. The AFM free energy density has the form $E_{\rm AFM}=\frac{M_{\rm s}}{\gamma}\{\omega_{\rm E}(\mathbf{m}^2-\mathbf{n}^2)-\frac{\omega_{\rm E}}{k_{\rm a}^2}[(\nabla\mathbf{m})^2-(\nabla\mathbf{n})^2]-\omega_{\rm A}(m_{\rm x}^2+n_{\rm x}^2)-2\omega_{\rm H}m_{\rm x}\}$. Here, $\omega_{\rm E}$ is the exchange frequency, $\omega_{\rm A}$ is the anisotropy frequency with easy-axis along $\mathbf{e}_{\rm x}$, $\omega_{\rm H}$ is the frequency describing the external magnetic field along $\mathbf{e}_{\rm x}$, $k_{\rm a}=2/a$, and $a$ is the unit cell length. The spatially varying spin orbit torques (SOTs) read $\mathbf{T}_{\rm m}=\gamma c_{\rm J}(x)(\mathbf{m}\times\mathbf{e}_{\rm x}\times\mathbf{m}+\mathbf{n}\times\mathbf{e}_{\rm x}\times\mathbf{n})$ and $\mathbf{T}_{\rm n}=\gamma c_{\rm J}(x)(\mathbf{n}\times\mathbf{e}_{\rm x}\times\mathbf{m}+\mathbf{m}\times\mathbf{e}_{\rm x}\times\mathbf{n})$. The AFM magnons are described by slight derivations $\mathbf{m}_{\rm s}=(0,\delta m_{\rm y},\delta m_{\rm z})$ and $\mathbf{n}_{\rm s}=(0,\delta n_{\rm y},\delta n_{\rm z})$ from the equilibrium $\mathbf{m}_0=(0,0,0)$ and $\mathbf{n}_0=(1,0,0)$. Substituting the magnon function and defining $\psi_{\rm m}=\delta m_{\rm y}-{\rm i}\delta m_{\rm z}$ and $\psi_{\rm n}=\delta n_{\rm y}-{\rm i}\delta n_{\rm z}$, the equation (S1) is reformulated in the coupled Helmholtz equations,

$$\begin{aligned}\psi_{\rm n}''(x)-(\frac{\omega_{\rm A}k_{\rm a}^2}{\omega_{\rm E}}-{\rm i}\frac{(\omega_{\rm J}(x)+\alpha\omega)k_{\rm a}^2}{\omega_{\rm E}})\psi_{\rm n}+\frac{(\omega-\omega_{\rm H})k_{\rm a}^2}{\omega_{\rm E}}\psi_{\rm m}&=0,\\ \psi_{\rm m}''(x)+(\frac{\omega_{\rm A}k_{\rm a}^2}{\omega_{\rm E}}+2k_{\rm a}^2-{\rm i}\frac{(\omega_{\rm J}(x)+\alpha\omega)k_{\rm a}^2}{\omega_{\rm E}})\psi_{\rm m}-\frac{(\omega-\omega_{\rm H})k_{\rm a}^2}{\omega_{\rm E}}\psi_{\rm n}&=0.\end{aligned}\tag{S2}$$

By setting forward ($+x$ direction) and backward ($-x$ direction) propagating magnons to in the form $\psi_{\rm n}=\delta n_{\rm y}-{\rm i}\delta n_{\rm z}=S_{\rm n}(x){\rm e}^{{\rm i}k_{\rm p}x}+R_{\rm n}(x){\rm e}^{-{\rm i}k_{\rm p}x}$ and eliminating $\psi_{\rm m}$, we deduce AFM magnonic equations of motion near the Bragg point as,

$$\begin{aligned}-{\rm i}R_{\rm n}'(x)+\delta_{\rm k}R_{\rm n}(x)&=\xi_{\rm n}S_{\rm n}(x),\\ {\rm i}S_{\rm n}'(x)+\delta_{\rm k}S_{\rm n}(x)&=-\xi_{\rm n}R_{\rm n}(x).\end{aligned}\tag{S3}$$

Then, the transfer matrix for AFM magnons is obtained as,

$$\begin{pmatrix}S(L)\\R(L)\end{pmatrix}=\begin{pmatrix}\cos(\beta_{\rm n}L)+{\rm i}\frac{\delta_{\rm k}}{\beta_{\rm n}}\sin(\beta_{\rm n}L) & {\rm i}\frac{\xi_{\rm n}}{\beta_{\rm n}}\sin(\beta_{\rm n}L)\\ {\rm i}\frac{\xi_{\rm n}}{\beta_{\rm n}}\sin(\beta_{\rm n}L) & \cos(\beta_{\rm n}L)-{\rm i}\frac{\delta_{\rm k}}{\beta_{\rm n}}\sin(\beta_{\rm n}L)\end{pmatrix}\begin{pmatrix}S(0)\\R(0)\end{pmatrix},\tag{S4}$$

Following notions are used: $A_{\rm n}=(\omega_{\rm A}/\omega_{\rm E}+1)k_{\rm a}^2$, $J_{\rm n}=k_{\rm a}^2\gamma c_{\rm A}/(\omega_{\rm E})$, $\xi_{\rm n}=\frac{A_{\rm n}J_{\rm n}}{2k_{\rm p}(k_{\rm a}^2-k_{\rm p}^2)}$, $\delta_{\rm k}=k_{\rm x}-k_{\rm p}$, $\beta_{\rm n}=\sqrt{\delta_{\rm k}^2+\xi_{\rm n}^2}$. Comparing to the ferromagnetic waveguide in the main text, one can replace $\beta$ and $\xi$ by $\beta_{\rm n}$ and $\xi_{\rm n}$ to obtain Eq. (S4) of AFM. The AFM magnon wavevector $k_{\rm x}$ is determined from the dispersion $\omega_{\pm}-\omega_{\rm H}=\pm\{(\omega_{\rm E}k_{\rm a}^2k_{\rm x}^2+\omega_{\rm A}-{\rm i}\alpha\omega)(2\omega_{\rm E}+\omega_{\rm A}-\omega_{\rm E}k_{\rm a}^2k_{\rm x}^2-{\rm i}\alpha\omega)\}^{1/2}$.

The magnon modes with $\omega_\pm$ correspond to the opposite circular polarizations. Without applying a magnetic field ($\omega_{\rm H} = 0$), the transfer matrices for two oppositely polarized magnons are degenerate, and thus opposite magnons are equally transmitted. A finite $\omega_{\rm H}$ lifts the degeneracy, and at the same Bragg point wavevector $k_{\rm p}$ opposite magnons with unequal frequencies obey different lasing and anti-lasing conditions. As demonstrated by Fig. S2 with a magnetic field in $+\mathbf{e}_{\rm x}$ direction, the lasing ($M_{22} = 0$) and anti-lasing ($M_{11} = 0$) conditions for right-hand polarized magnon (with $\omega_+$) are different from those for left-hand polarized magnon (with $\omega_-$). At $c_{\rm A} = 268$ A/m, we reach the lasing condition for left-hand polarized magnon, which is below the lasing condition $c_{\rm A} = 292$ A/m of right-hand polarized magnon, allowing for selective amplification of left-hand magnon with frequency 0.24 THz. Besides, exploiting the different anti-lasing conditions, it is possible to selectively absorb one of two opposite magnon modes.

## REFERENCES


[1] R. Cheng, D. Xiao, and A. Brataas, *Terahertz antiferromagnetic spin hall nano-oscillator,* Phys. Rev. Lett. **116**, 207603 (2016).

[2] O. Johansen, H. Skarsvåg, and A. Brataas, *Spin-transfer antiferromagnetic resonance,* Phys. Rev. B **97**, 054423 (2018).

[3] V. Baltz, A. Manchon, M. Tsoi, T. Moriyama, T. Ono, and Y. Tserkovnyak, *Antiferromagnetic spintronics,* Rev. Mod. Phys. **90**, 015005 (2018).

[4] X.-g. Wang, Y.-Z. Nie, L. Chotorlishvili, Q.-l. Xia, J. Berakdar, and G.-h. Guo, *Electron-magnon spin conversion and magnonic spin pumping in an antiferromagnet/heavy metal heterostructure,* Phys. Rev. B **103**, 064404 (2021).
